# Supplementary material for: Do Language Models Understand Igbo Culture? Beyond Multiple Choice
Source: arXiv:2610.35168 source file (2026-10-27)
Supplement: Supplementary file 1 [file appendix_repetition.tex]

\begin{figure*}[t]
\centering\small
\begin{tabular}{@{}L{0.485\textwidth}@{\hspace{0.03\textwidth}}L{0.485\textwidth}@{}}
\toprule
\textbf{LLaMA 3.1 8B, Type 2, question 1 (Family and Kinship)}\newline\textit{Ọnwụma bụ aha Igbo nke pụrụ ịgụ n\textquotesingle{}ụdị dị iche iche. Ọ nwụrụ n\textquotesingle{}ụdị dị ka Ọnwụma Ọjọọ, Ọnwụma Ọjọọ Ọjọọ, Ọnwụma Ọjọọ Ọjọọ Ọjọọ, Ọnwụma Ọjọọ Ọjọọ Ọjọọ Ọjọọ, Ọnwụma Ọjọọ Ọjọọ Ọjọọ Ọjọọ Ọjọọ, Ọnwụma Ọjọọ …} & \textbf{LLaMA 3 8B Lite, Type 2, question 1 (Family and Kinship)}\newline\textit{Onye agha agha agha agha agha agha agha agha agha agha agha agha agha agha agha agha agha agha agha agha agha agha agha agha agha agha agha agha agha agha agha agha agha agha agha agha agha agha agha …} \\
\midrule
\textbf{GPT-OSS 20B, Type 2, question 5 (Family and Kinship)}\newline\textit{Nke a bụ ihe a na-ahụkarị: nwa ọhụrụ nwere àgwà ma ọ bụ àgwà dị iche, dịka ịma mma ma ọ bụ obi ike, nke yiri nke nna nna ahụ. Ọtụtụ mgbe, a na-ahụkwa akara anụ ahụ dịka àgwà ma ọ bụ àgwà dị iche, …} & \textbf{LLaMA 3.1 8B, Type 3, question 1 (Family and Kinship)}\newline\textit{Nkọwa nke ọnwụ ụmụ ọhụrụ na ịgụ aha ndị Igbo gbasara ọnwụ ụmụ ọhụrụ: 1. Ọnwụ ụmụ ọhụrụ bụ ihe a na-egosi mgbe ndị nne na nna gụrụ nwa aha ịma aka dị ka Ọnwụma. Aha Ọnwụma bụ aha nke a na-egosi ọnwụ …} \\
\midrule
\textbf{AfriqueQwen 14B, Type 3, question 5 (Family and Kinship)}\newline\textit{N\textquotesingle{}ọdịnala ụfọdụ, a na-ekwu na nna nna nwụrụ anwụ nwere ike ịlaghachi n\textquotesingle{}ahụ nwa ọhụrụ, a na-akpọkarị nke a \textquotedbl{}reincarnation.\textquotedbl{} Otú ọ dị, enweghị ihe akaebe sayensị siri ike nke na-akwado nkwupụta a. …} & \textbf{LLaMA 3.3 70B, Type 3, question 4 (Proverbs and Oral Tradition)}\newline\textit{Echiche nkà ihe ọmụma gbasara ihe a na-akọwa na \textquotedbl{}Ebe nwa na ebe akwa na alu eka, nnenye anoghulio nu nnanya a nolaa\textquotedbl{} bụ na ọ bụ eziokwu na mmadụ niile nwere ebe ha si, ebe ha bụrụ nwa, na ebe ha …} \\
\bottomrule
\end{tabular}
\caption{Repetition-loop failures in open-ended generation under Igbo prompting. Each cell is a verbatim excerpt from a model response in the human-evaluation sample, truncated where marked with an ellipsis. The annotator labelled all six responses as Model Breakdown and Repetition.}
\label{fig:repetition}
\end{figure*}
